# Supplementary material for: A Reexamination of the Communication Bandwidth Cost Analysis of A Parallel Recursive Algorithm for Solving Triangular Systems of Linear Equations
Source: arXiv:2407.00871 source file (2024-04-10)
Supplement: Supplementary file 1 [file appendix.tex]

\secput{app}{Artifact Description}
\punt{% begin punt
Following is some paragraph for a research paper. Please polish it appropriate. Making it concise, clear, and to-the-point. You should NOT omit any main information. You should also keep all the Latex commands of the input.
}% end punt

In the main text of this 2-page comment paper, we provide citations for all evidence and sources. The original paper by Wicky et al. \cite{WickySoHo17} can be accessed at the ACM Digital Library.
